# Supplementary material for: Mode jumping MCMC for Bayesian variable selection in GLMM
Source: arXiv:1604.06398 source file (2018-06-07)
Supplement: Supplementary file 1 [file appendix.tex]

\documentclass[10pt,a4paper]{article}
\usepackage[utf8]{inputenc}
\usepackage{amsmath}
\usepackage{amsfonts}
\usepackage{amssymb}
\usepackage{adjustbox}
\usepackage{graphicx}
\usepackage{enumerate}
\usepackage{comment}
\usepackage{bbold}
\usepackage{float}
\usepackage{algorithm}% http://ctan.org/pkg/algorithms
\usepackage{algpseudocode}% http://ctan.org/pkg/algorithmicx
\usepackage{natbib}
\usepackage[colorlinks=true,
            linkcolor=blue,
            urlcolor=blue,
            citecolor=blue]{hyperref}

\usepackage{array}
\newcolumntype{H}{>{\setbox0=\hbox\bgroup}c<{\egroup}@{}}

\usepackage{xr}
\externaldocument{main}

\usepackage{chngcntr}

\addtolength{\oddsidemargin}{-.75in}
\addtolength{\evensidemargin}{-.75in}
\addtolength{\textwidth}{1.5in}
\addtolength{\textheight}{1.3in}
\addtolength{\topmargin}{-.8in}

\begin{document}

\bibliographystyle{apalike}

\counterwithin{equation}{section}
\counterwithin{table}{section}
\counterwithin{algorithm}{section}
\input{appendix_main.tex}

\newpage 

\bibliography{ref}

\end{document}
